# Supplementary material for: UniGRPO: Unified Policy Optimization for Reasoning-Driven Visual Generation
Source: arXiv:2603.23500 source file (2026-03-24)
Supplement: Supplementary file 1 [file appendix.tex]

\section{Hello World}
%\subsection{Hello World}
